# Supplementary material for: Mitigating Preference Leakage via Strict Estimator Separation for Normative Generative Ranking
Source: arXiv:2602.20800 source file (2026-02-25)
Supplement: Supplementary file 1 [file appendix_main_setting.tex]

\appendix
\section{Evaluation Configuration and Robustness}
\label{app:main_setting}

\subsection{Fixed Evaluation Configuration (q70, $k{=}5$)}
\label{app:main_setting_spec}

\paragraph{Intersection pool (q70 setting).}
On the cleaned GEMMA dataset ($N=33{,}052$; 343 queries), the intersection pool $(y_A \cap y_B)$ retains 17{,}965 stories and all queries remain eligible at $k{=}5$.
Over the pooled q70 \textbf{test} query$\times$seed rows ($n{=}700$), intersection pool sizes satisfy
$\min/\mathrm{median}/\mathrm{mean}/\max = 10/51/51.70/106$. These statistics are computed over the pooled test query$\times$seed rows ($n{=}700$) and therefore differ slightly from the across-query distribution reported in Table~\ref{tab:pool_stats_gemma} (343 queries).

\paragraph{Leakage-free query-level splits and reporting.}
We split at the \textbf{query level} so each \texttt{query\_id} (and its full candidate pool) appears in exactly one of train/dev/test. Using 10 seeds, each split contains 239/34/70 train/dev/test queries. We compute metrics per query and macro-average over the 70 test queries to obtain a seed-level score, then report mean$\pm$std over 10 seeds.

\subsection{Candidate Pool Statistics}
\label{app:pool_stats}

Using the cleaned GEMMA dataset ($N=33{,}052$), the intersection pool ($y_A \cap y_B$) contains 17{,}965 stories across 343 eligible queries after filtering out null or invalid judge outputs.
Table~\ref{tab:pool_stats_gemma} summarises the distribution of intersection pool sizes across eligible queries.

\begin{table}[t]
\centering
\small
\setlength{\tabcolsep}{6pt}
\caption{Intersection candidate-pool statistics on the cleaned GEMMA dataset (343 queries).}
\label{tab:pool_stats_gemma}
\begin{tabular}{lrrrr}
\toprule
\textbf{Pool} & \textbf{min} & \textbf{median} & \textbf{mean} & \textbf{max} \\
\midrule
$|\mathcal{S}_q^{\cap}|$ & 10 & 52 & 52.38 & 106 \\
\bottomrule
\end{tabular}
\end{table}

\subsection{Pre-judging Candidate Pool Density}
\label{app:prejudging_density}

Before judging, each structured query $q=(\text{age},\text{moral},\text{culture})$ defines a candidate pool $\mathcal{S}_q$. On the cleaned dataset ($N=33{,}052$ stories; 343 queries), candidate pools are dense, with the following pool-size statistics computed directly from the story file.

\begin{table}[t]
\centering
\small
\setlength{\tabcolsep}{6pt}
\caption{Pre-judging candidate pool-size statistics computed from the cleaned story file (343 queries).}
\label{tab:prejudging_pool_stats}
\begin{tabular}{lrrrr}
\toprule
\textbf{Pool} & \textbf{min} & \textbf{median} & \textbf{mean} & \textbf{max} \\
\midrule
$|\mathcal{S}_q|$ & 33 & 96 & 96.36 & 161 \\
\bottomrule
\end{tabular}
\end{table}

\subsection{Sensitivity to Candidate Pool Size}
\label{app:pool_sensitivity}

We analyze whether conclusions depend on candidate-pool size by binning \emph{test queries} (per seed) based on $|\mathcal{S}_q^{\cap}|$ into Small ($\leq 35$), Medium (36--50), and Large ($>50$).
Values are mean$\pm$std over 10 seeds (seed-level means within each bin). 
B-Score is omitted here because bin-level values were not available in our stored outputs.

\begin{table}[t]
\centering
\caption{Pool-size sensitivity (nDCG@5 at $k{=}5$) on q70 test queries.}
\label{tab:pool_sensitivity_ndcg5}
\small
\setlength{\tabcolsep}{5pt}

\begin{tabular}{lccc}
\toprule
\textbf{Method} & \textbf{Small} & \textbf{Medium} & \textbf{Large} \\
\midrule
Random & 0.5917 $\pm$ 0.0413 & 0.5549 $\pm$ 0.0421 & 0.5668 $\pm$ 0.0299 \\
BM25 & 0.6067 $\pm$ 0.0610 & 0.6068 $\pm$ 0.0527 & 0.6226 $\pm$ 0.0551 \\
BGE-M3 & 0.6991 $\pm$ 0.0729 & 0.6244 $\pm$ 0.0667 & 0.6355 $\pm$ 0.0425 \\
B-Score (Judge B) & -- & -- & -- \\
Neural (pointwise; $y_B$) & 0.5876 $\pm$ 0.0425 & 0.5588 $\pm$ 0.0435 & 0.5763 $\pm$ 0.0411 \\
Neural (pairwise; $y_B$) & 0.5820 $\pm$ 0.0435 & 0.5520 $\pm$ 0.0581 & 0.5704 $\pm$ 0.0384 \\
RankGPT-direct (Mistral) & 0.5791 $\pm$ 0.0411 & 0.5306 $\pm$ 0.0467 & 0.5642 $\pm$ 0.0320 \\
\bottomrule
\end{tabular}
\end{table}

\subsection{Sensitivity to Cutoff $k$}
\label{app:k_sensitivity}

We vary the evaluation cutoff $k \in \{1,3,5,10\}$ while keeping the q70 setup fixed: the same 10 query-level train/dev/test splits, and the same intersection candidate pools.
Figure~\ref{fig:k_sensitivity_ndcg} reports nDCG@$k$ (mean$\pm$std over 10 seeds) for all rankers, highlighting robustness to the choice of cutoff.

\begin{figure}[t!]
\centering
\includegraphics[width=0.88\linewidth]{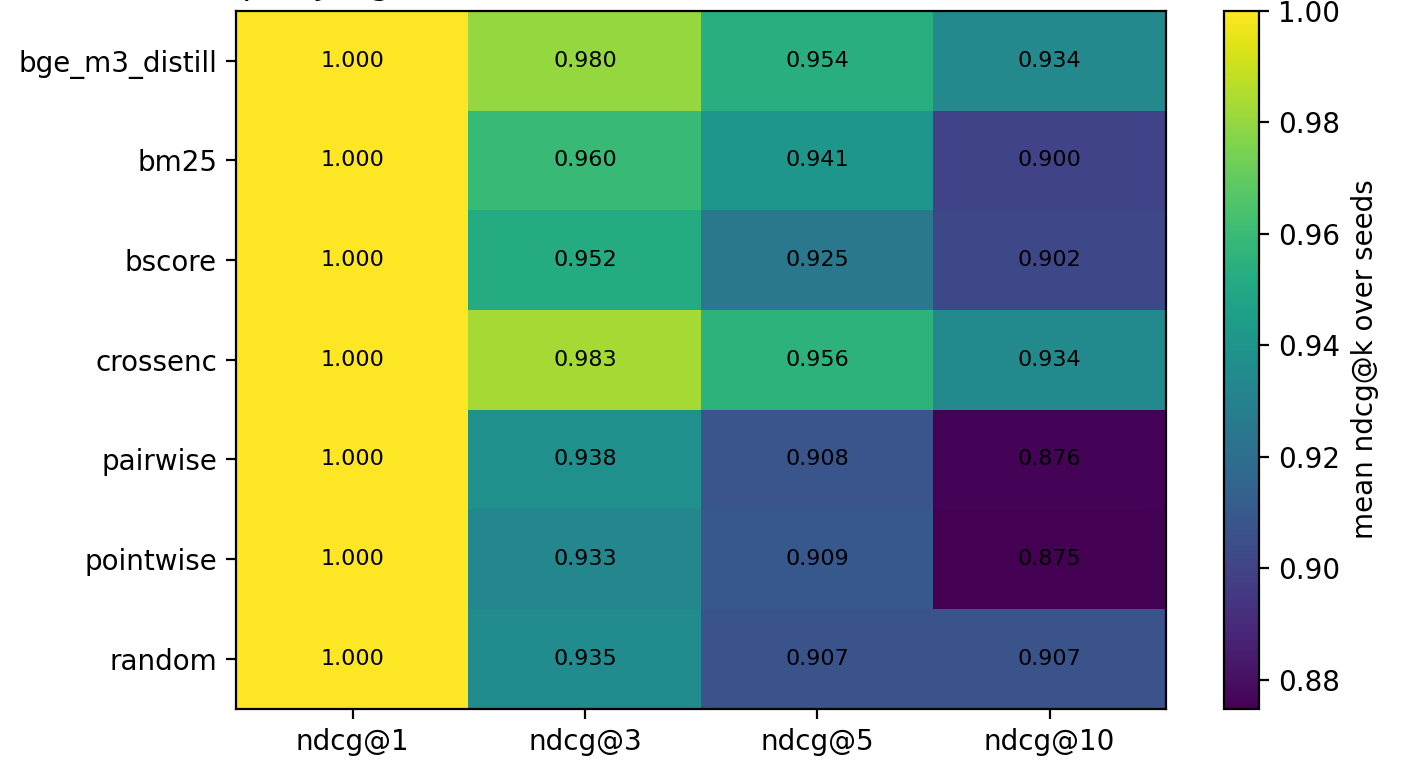}
\caption{Sensitivity to the evaluation cutoff $k$ on q70 (nDCG@$k$; mean$\pm$std over 10 seeds; same splits and candidate pool).}
\label{fig:k_sensitivity_ndcg}
\end{figure}

\subsection{Reproducibility Artifacts}
\label{app:repro}

For each seed, we store the query-level split manifest, per-method prediction JSONL files, and aggregated result summaries (including LaTeX-ready table rows). We also store pooled query$\times$seed rows used for paired significance testing.

All runs fix random seeds, decoding/truncation settings, and the intersection candidate pools $(y_A \cap y_B)$ for all downstream stages. Story generation is performed once using stochastic decoding with a fixed seed, after which all judging, ranking, and evaluation experiments operate deterministically on the frozen generated corpus. As a result, methods differ only by the ranking function applied to identical candidate pools.
Experiments are executed fully offline with local checkpoints, and model identifiers and key hyperparameters are recorded in the written result files.

\section{External Validity}
\label{app:external_validity}

\subsection{SS-GEN}
\label{app:ssgen}

We run an out-of-domain sanity check on \textsc{SS-GEN} (\emph{SS-GEN: A Social Story Generation Framework with Large Language Models})~\cite{li2024ssgen} by uniformly sampling $N{=}500$ instances with a fixed random seed (42) and scoring the same subset independently with Judge~A and Judge~B under the same JSON-only constraint.
Judge~A yields 4 null outputs (0.8\%), while Judge~B yields 35 null outputs (7.0\%).
Agreement is computed over the intersection of instances with valid scores from both judges ($n{=}462$), yielding low correlation (Spearman $\rho{=}0.0458$, Kendall $\tau{=}0.0445$).

\begin{table}[t]
\centering
\small
\setlength{\tabcolsep}{6pt}
\begin{tabular}{lcccc}
\toprule
Dataset (subset) & $N$ & Null-rate (A) & Null-rate (B) & Agreement on valid intersection \\
\midrule
\textsc{SS-GEN} (seed=42) & 500 & 0.8\% & 7.0\% & $\rho{=}0.0458$, $\tau{=}0.0445$ \\
\bottomrule
\end{tabular}
\caption{\textsc{SS-GEN} external sanity check summary on a uniformly sampled subset. Agreement is computed on the intersection of instances with valid scores from both judges.}
\label{tab:ssgen_sanity}
\end{table}

\begin{table}[t]
\centering
\small
\setlength{\tabcolsep}{6pt}
\begin{tabular}{lrrrrrr}
\toprule
Judge & Null & 1 & 2 & 3 & 4 & 5 \\
\midrule
A & 4  & 164 & 3  & 323 & 2 & 4 \\
B & 35 & 6   & 37 & 394 & 6 & 22 \\
\bottomrule
\end{tabular}
\caption{Score distributions on the sampled \textsc{SS-GEN} subset ($N{=}500$).}
\label{tab:ssgen_label_dist}
\end{table}

\subsection{Moral Stories}
\label{app:external_moralstories}

To assess external validity on a norm-focused dataset, we run the same two-judge pipeline on \textsc{Moral Stories} (500 instances)~\cite{emelin2021moral}.
We treat the norm statement as the query and score each narrative using the same discrete 1--5 rubric and JSON-only constraint.
Judge~A produces valid scores for 469/500 stories (93.8\%), while Judge~B produces valid scores for 500/500 (100\%).
On the 469 stories with both scores available, inter-judge agreement is strong: Spearman's $\rho=0.653$ ($p=2.35\times10^{-58}$) and Kendall's $\tau=0.594$ ($p=6.34\times10^{-46}$), with an exact-score match rate of 292/469 (62.3\%).

\begin{table}[t]
\centering
\small
\setlength{\tabcolsep}{6pt}
\begin{tabular}{lrrrr}
\toprule
Dataset (subset) & $N$ & Valid (A) & Valid (B) & Agreement on valid intersection \\
\midrule
\textsc{Moral Stories} & 500 & 469 & 500 & $\rho{=}0.653$, $\tau{=}0.594$ \\
\bottomrule
\end{tabular}
\caption{\textsc{Moral Stories} external sanity check summary. Agreement is computed on the intersection of instances with valid scores from both judges.}
\label{tab:moralstories_sanity}
\end{table}
